# Supplementary material for: MARE: Multi-Agents Collaboration Framework for Requirements Engineering
Source: arXiv:2405.03256 source file (2024-05-06)
Supplement: Supplementary file 1 [file 9appendix.tex]

\appendix

\subsection{The prompt for every action} \label{prompt}

\subsection{The Template for draft and SRS} \label{template}

\subsection{The detail about five new evaluation cases} \label{cases}
